# Supplementary material for: Bastion: Budget-Aware Speculative Decoding with Tree-structured Block Diffusion Drafting
Source: arXiv:2605.29727 source file (2026-10-28)
Supplement: Supplementary file 1 [file addtional_gpu_model_result.tex]

\begin{table*}[!htbp]
\centering
\caption{\textbf{Additional results on Nvidia A6000 and RTX PRO 6000 Blackwell (B6000).} Speedup and AAL ($\tau$) for Qwen3-4B, Qwen3-8B, and Llama-3.1-8B-Instruct at temperature $T=0$. For the baselines, the tree budget size of EAGLE-3 is set to 60. The block size of DFlash is 16 for Qwen3-4B and Qwen3-8B, and 10 for Llama-3.1-8B-Instruct. \textbf{Bold} indicates the highest value within each (model, benchmark) pair.}
\label{tab:add_res_all}
\small
\setlength{\tabcolsep}{1pt}

\begin{subtable}{\textwidth}
\centering
\caption{Qwen3-4B}
\label{tab:add_res_qwen3_4b}
\resizebox{\textwidth}{!}{
\begin{tabular}{c | c | *{3}{c c} | *{3}{c c} |*{2}{c c} | *{1}{c c}}
\toprule
\multirow{2.5}{*}{\textbf{GPU}} & \multirow{2.5}{*}{\textbf{Method}} & \multicolumn{2}{c}{\textbf{GSM8K}} & \multicolumn{2}{c}{\textbf{MATH500}} & \multicolumn{2}{c}{\textbf{AIME25}} & \multicolumn{2}{|c}{\textbf{HumanEval}} & \multicolumn{2}{c}{\textbf{MBPP}} & \multicolumn{2}{c}{\textbf{LCB}} & \multicolumn{2}{|c}{\textbf{MT-Bench}} & \multicolumn{2}{c}{\textbf{Alpaca}} & \multicolumn{2}{|c}{\textbf{Average}} \\
\cmidrule(lr){3-4} \cmidrule(lr){5-6} \cmidrule(lr){7-8} \cmidrule(lr){9-10} \cmidrule(lr){11-12} \cmidrule(lr){13-14} \cmidrule(lr){15-16} \cmidrule(lr){17-18} \cmidrule(lr){19-20}
& & Speedup & $\tau$ & Speedup & $\tau$ & Speedup & $\tau$ & Speedup & $\tau$ & Speedup & $\tau$ & Speedup & $\tau$ & Speedup & $\tau$ & Speedup & $\tau$ & Speedup & $\tau$ \\
\midrule
& EAGLE-3 & $3.26\times$ & 2.82 & $3.09\times$ & 2.57 & $3.01\times$ & 2.56 & $2.92\times$ & 2.49 & $2.82\times$ & 2.43 & $2.61\times$ & 2.30 & $2.78\times$ & 2.49 & $2.49\times$ & 2.21 & $2.87\times$ & 2.48 \\
& DFlash & $5.06\times$ & 6.43 & $6.02\times$ & 8.04 & $5.76\times$ & 7.48 & $5.06\times$ & 6.70 & $4.69\times$ & 6.31 & $5.44\times$ & 7.29 & $2.77\times$ & 4.59 & $2.01\times$ & 2.90 & $4.60\times$ & 6.22 \\
\rowcolor{blue!10} \cellcolor{white} \multirow{-3}{*}{A6000} & \textbf{\algo} & $\mathbf{7.62\times}$ & \textbf{8.99} & $\mathbf{8.50\times}$ & \textbf{10.45} & $\mathbf{7.64\times}$ & \textbf{9.47} & $\mathbf{7.82\times}$ & \textbf{9.28} & $\mathbf{7.47\times}$ & \textbf{8.97} & $\mathbf{7.61\times}$ & \textbf{9.54} & $\mathbf{4.67\times}$ & \textbf{6.61} & $\mathbf{3.60\times}$ & \textbf{4.60} & $\mathbf{6.87\times}$ & \textbf{8.49} \\
\cmidrule{1-20}
& EAGLE-3 & $3.11\times$ & 2.82 & $2.88\times$ & 2.58 & $2.83\times$ & 2.52 & $2.80\times$ & 2.50 & $2.70\times$ & 2.41 & $2.56\times$ & 2.28 & $2.81\times$ & 2.50 & $2.48\times$ & 2.23 & $2.77\times$ & 2.48 \\
& DFlash & $4.85\times$ & 6.49 & $5.62\times$ & 7.83 & $5.51\times$ & 7.40 & $4.86\times$ & 6.67 & $4.42\times$ & 6.15 & $5.02\times$ & 6.93 & $2.74\times$ & 4.42 & $2.06\times$ & 3.10 & $4.39\times$ & 6.12 \\
\rowcolor{blue!10} \cellcolor{white} \multirow{-3}{*}{B6000} & \textbf{\algo} & $\mathbf{6.69\times}$ & \textbf{9.05} & $\mathbf{7.41\times}$ & \textbf{10.52} & $\mathbf{6.80\times}$ & \textbf{9.56} & $\mathbf{6.70\times}$ & \textbf{9.42} & $\mathbf{6.49\times}$ & \textbf{9.16} & $\mathbf{7.20\times}$ & \textbf{9.75} & $\mathbf{4.12\times}$ & \textbf{6.50} & $\mathbf{3.08\times}$ & \textbf{4.68} & $\mathbf{6.06\times}$ & \textbf{8.58} \\
\bottomrule
\end{tabular}
}
\end{subtable}

\vspace{0.8em}

\begin{subtable}{\textwidth}
\centering
\caption{Qwen3-8B}
\label{tab:add_res_qwen3_8b}
\resizebox{\textwidth}{!}{
\begin{tabular}{c | c | *{3}{c c} | *{3}{c c} |*{2}{c c} | *{1}{c c}}
\toprule
\multirow{2.5}{*}{\textbf{GPU}} & \multirow{2.5}{*}{\textbf{Method}} & \multicolumn{2}{c}{\textbf{GSM8K}} & \multicolumn{2}{c}{\textbf{MATH500}} & \multicolumn{2}{c}{\textbf{AIME25}} & \multicolumn{2}{|c}{\textbf{HumanEval}} & \multicolumn{2}{c}{\textbf{MBPP}} & \multicolumn{2}{c}{\textbf{LCB}} & \multicolumn{2}{|c}{\textbf{MT-Bench}} & \multicolumn{2}{c}{\textbf{Alpaca}} & \multicolumn{2}{|c}{\textbf{Average}} \\
\cmidrule(lr){3-4} \cmidrule(lr){5-6} \cmidrule(lr){7-8} \cmidrule(lr){9-10} \cmidrule(lr){11-12} \cmidrule(lr){13-14} \cmidrule(lr){15-16} \cmidrule(lr){17-18} \cmidrule(lr){19-20}
& & Speedup & $\tau$ & Speedup & $\tau$ & Speedup & $\tau$ & Speedup & $\tau$ & Speedup & $\tau$ & Speedup & $\tau$ & Speedup & $\tau$ & Speedup & $\tau$ & Speedup & $\tau$ \\
\midrule
& EAGLE-3 & $2.97\times$ & 2.70 & $2.79\times$ & 2.52 & $2.68\times$ & 2.50 & $2.86\times$ & 2.63 & $2.61\times$ & 2.26 & $2.19\times$ & 2.02 & $2.37\times$ & 2.23 & $2.07\times$ & 1.82 & $2.57\times$ & 2.34 \\
& DFlash & $4.87\times$ & 6.53 & $5.77\times$ & 8.06 & $5.31\times$ & 7.06 & $4.85\times$ & 6.69 & $4.32\times$ & 5.98 & $4.98\times$ & 7.31 & $2.54\times$ & 4.47 & $2.07\times$ & 3.15 & $4.34\times$ & 6.16 \\
\rowcolor{blue!10} \cellcolor{white} \multirow{-3}{*}{A6000} & \textbf{\algo} & $\mathbf{6.95\times}$ & \textbf{8.47} & $\mathbf{7.86\times}$ & \textbf{10.19} & $\mathbf{6.79\times}$ & \textbf{9.06} & $\mathbf{7.26\times}$ & \textbf{9.21} & $\mathbf{6.77\times}$ & \textbf{8.43} & $\mathbf{7.07\times}$ & \textbf{9.79} & $\mathbf{3.98\times}$ & \textbf{6.15} & $\mathbf{3.35\times}$ & \textbf{4.50} & $\mathbf{6.25\times}$ & \textbf{8.23} \\
\cmidrule{1-20}
& EAGLE-3 & $3.03\times$ & 2.71 & $2.79\times$ & 2.51 & $2.80\times$ & 2.52 & $2.87\times$ & 2.61 & $2.61\times$ & 2.24 & $2.27\times$ & 2.00 & $2.46\times$ & 2.21 & $2.16\times$ & 1.83 & $2.62\times$ & 2.33 \\
& DFlash & $4.86\times$ & 6.57 & $5.62\times$ & 7.92 & $5.36\times$ & 7.22 & $4.63\times$ & 6.53 & $4.40\times$ & 6.03 & $5.04\times$ & 7.17 & $2.60\times$ & 4.31 & $2.09\times$ & 3.10 & $4.33\times$ & 6.11 \\
\rowcolor{blue!10} \cellcolor{white} \multirow{-3}{*}{B6000} & \textbf{\algo} & $\mathbf{6.79\times}$ & \textbf{8.32} & $\mathbf{7.79\times}$ & \textbf{9.94} & $\mathbf{7.35\times}$ & \textbf{9.27} & $\mathbf{7.02\times}$ & \textbf{8.84} & $\mathbf{6.52\times}$ & \textbf{8.13} & $\mathbf{7.41\times}$ & \textbf{9.69} & $\mathbf{4.11\times}$ & \textbf{5.92} & $\mathbf{3.39\times}$ & \textbf{4.40} & $\mathbf{6.30\times}$ & \textbf{8.06} \\
\bottomrule
\end{tabular}
}
\end{subtable}

\vspace{0.8em}

\begin{subtable}{\textwidth}
\centering
\caption{Llama-3.1-8B-Instruct}
\label{tab:add_res_llama3_1_8b_instruct}
\resizebox{\textwidth}{!}{
\begin{tabular}{c | c | *{3}{c c} | *{3}{c c} |*{2}{c c} | *{1}{c c}}
\toprule
\multirow{2.5}{*}{\textbf{GPU}} & \multirow{2.5}{*}{\textbf{Method}} & \multicolumn{2}{c}{\textbf{GSM8K}} & \multicolumn{2}{c}{\textbf{MATH500}} & \multicolumn{2}{c}{\textbf{AIME25}} & \multicolumn{2}{|c}{\textbf{HumanEval}} & \multicolumn{2}{c}{\textbf{MBPP}} & \multicolumn{2}{c}{\textbf{LCB}} & \multicolumn{2}{|c}{\textbf{MT-Bench}} & \multicolumn{2}{c}{\textbf{Alpaca}} & \multicolumn{2}{|c}{\textbf{Average}} \\
\cmidrule(lr){3-4} \cmidrule(lr){5-6} \cmidrule(lr){7-8} \cmidrule(lr){9-10} \cmidrule(lr){11-12} \cmidrule(lr){13-14} \cmidrule(lr){15-16} \cmidrule(lr){17-18} \cmidrule(lr){19-20}
& & Speedup & $\tau$ & Speedup & $\tau$ & Speedup & $\tau$ & Speedup & $\tau$ & Speedup & $\tau$ & Speedup & $\tau$ & Speedup & $\tau$ & Speedup & $\tau$ & Speedup & $\tau$ \\
\midrule
& EAGLE-3 & $2.95\times$ & 3.26 & $2.55\times$ & 2.73 & $2.47\times$ & 2.74 & $3.00\times$ & 3.32 & $3.03\times$ & 3.30 & $2.23\times$ & 2.47 & $2.52\times$ & 2.94 & $2.35\times$ & 2.68 & $2.64\times$ & 2.93 \\
& DFlash & $3.29\times$ & 4.34 & $3.08\times$ & 4.19 & $3.48\times$ & 4.80 & $3.67\times$ & 4.86 & $3.93\times$ & 5.25 & $2.85\times$ & 3.79 & $2.78\times$ & 3.96 & $2.47\times$ & 3.44 & $3.19\times$ & 4.33 \\
\rowcolor{blue!10} \cellcolor{white} \multirow{-3}{*}{A6000} & \textbf{\algo} & $\mathbf{4.66\times}$ & \textbf{5.55} & $\mathbf{4.36\times}$ & \textbf{5.38} & $\mathbf{4.54\times}$ & \textbf{5.82} & $\mathbf{5.18\times}$ & \textbf{6.20} & $\mathbf{5.46\times}$ & \textbf{6.51} & $\mathbf{3.91\times}$ & \textbf{4.88} & $\mathbf{3.99\times}$ & \textbf{5.09} & $\mathbf{3.77\times}$ & \textbf{4.62} & $\mathbf{4.48\times}$ & \textbf{5.51} \\
\cmidrule{1-20}
& EAGLE-3 & $2.82\times$ & 3.25 & $2.54\times$ & 2.71 & $2.42\times$ & 2.62 & $2.99\times$ & 3.29 & $2.96\times$ & 3.30 & $2.27\times$ & 2.45 & $2.56\times$ & 2.95 & $2.37\times$ & 2.68 & $2.62\times$ & 2.91 \\
& DFlash & $3.09\times$ & 4.37 & $2.96\times$ & 4.29 & $3.13\times$ & 4.50 & $3.45\times$ & 4.91 & $3.66\times$ & 5.08 & $2.81\times$ & 3.94 & $2.65\times$ & 4.05 & $2.35\times$ & 3.48 & $3.01\times$ & 4.33 \\
\rowcolor{blue!10} \cellcolor{white} \multirow{-3}{*}{B6000} & \textbf{\algo} & $\mathbf{4.63\times}$ & \textbf{5.89} & $\mathbf{4.27\times}$ & \textbf{5.71} & $\mathbf{4.48\times}$ & \textbf{6.14} & $\mathbf{5.05\times}$ & \textbf{6.59} & $\mathbf{5.38\times}$ & \textbf{6.80} & $\mathbf{3.92\times}$ & \textbf{5.19} & $\mathbf{3.89\times}$ & \textbf{5.36} & $\mathbf{3.73\times}$ & \textbf{4.83} & $\mathbf{4.42\times}$ & \textbf{5.81} \\
\bottomrule
\end{tabular}
}
\end{subtable}

\end{table*}
